# Supplementary material for: Arbitrary-Scale Image Synthesis
Source: arXiv:2204.02273 source file (2022-04-05)
Supplement: Supplementary file 1 [file appendix.tex]

\section{Appendix}

\begin{figure*}[t]
    \centering%
    \begin{tabular}{ccc}
         \includegraphics[width=0.30\linewidth, trim=30 120 580 40, clip]{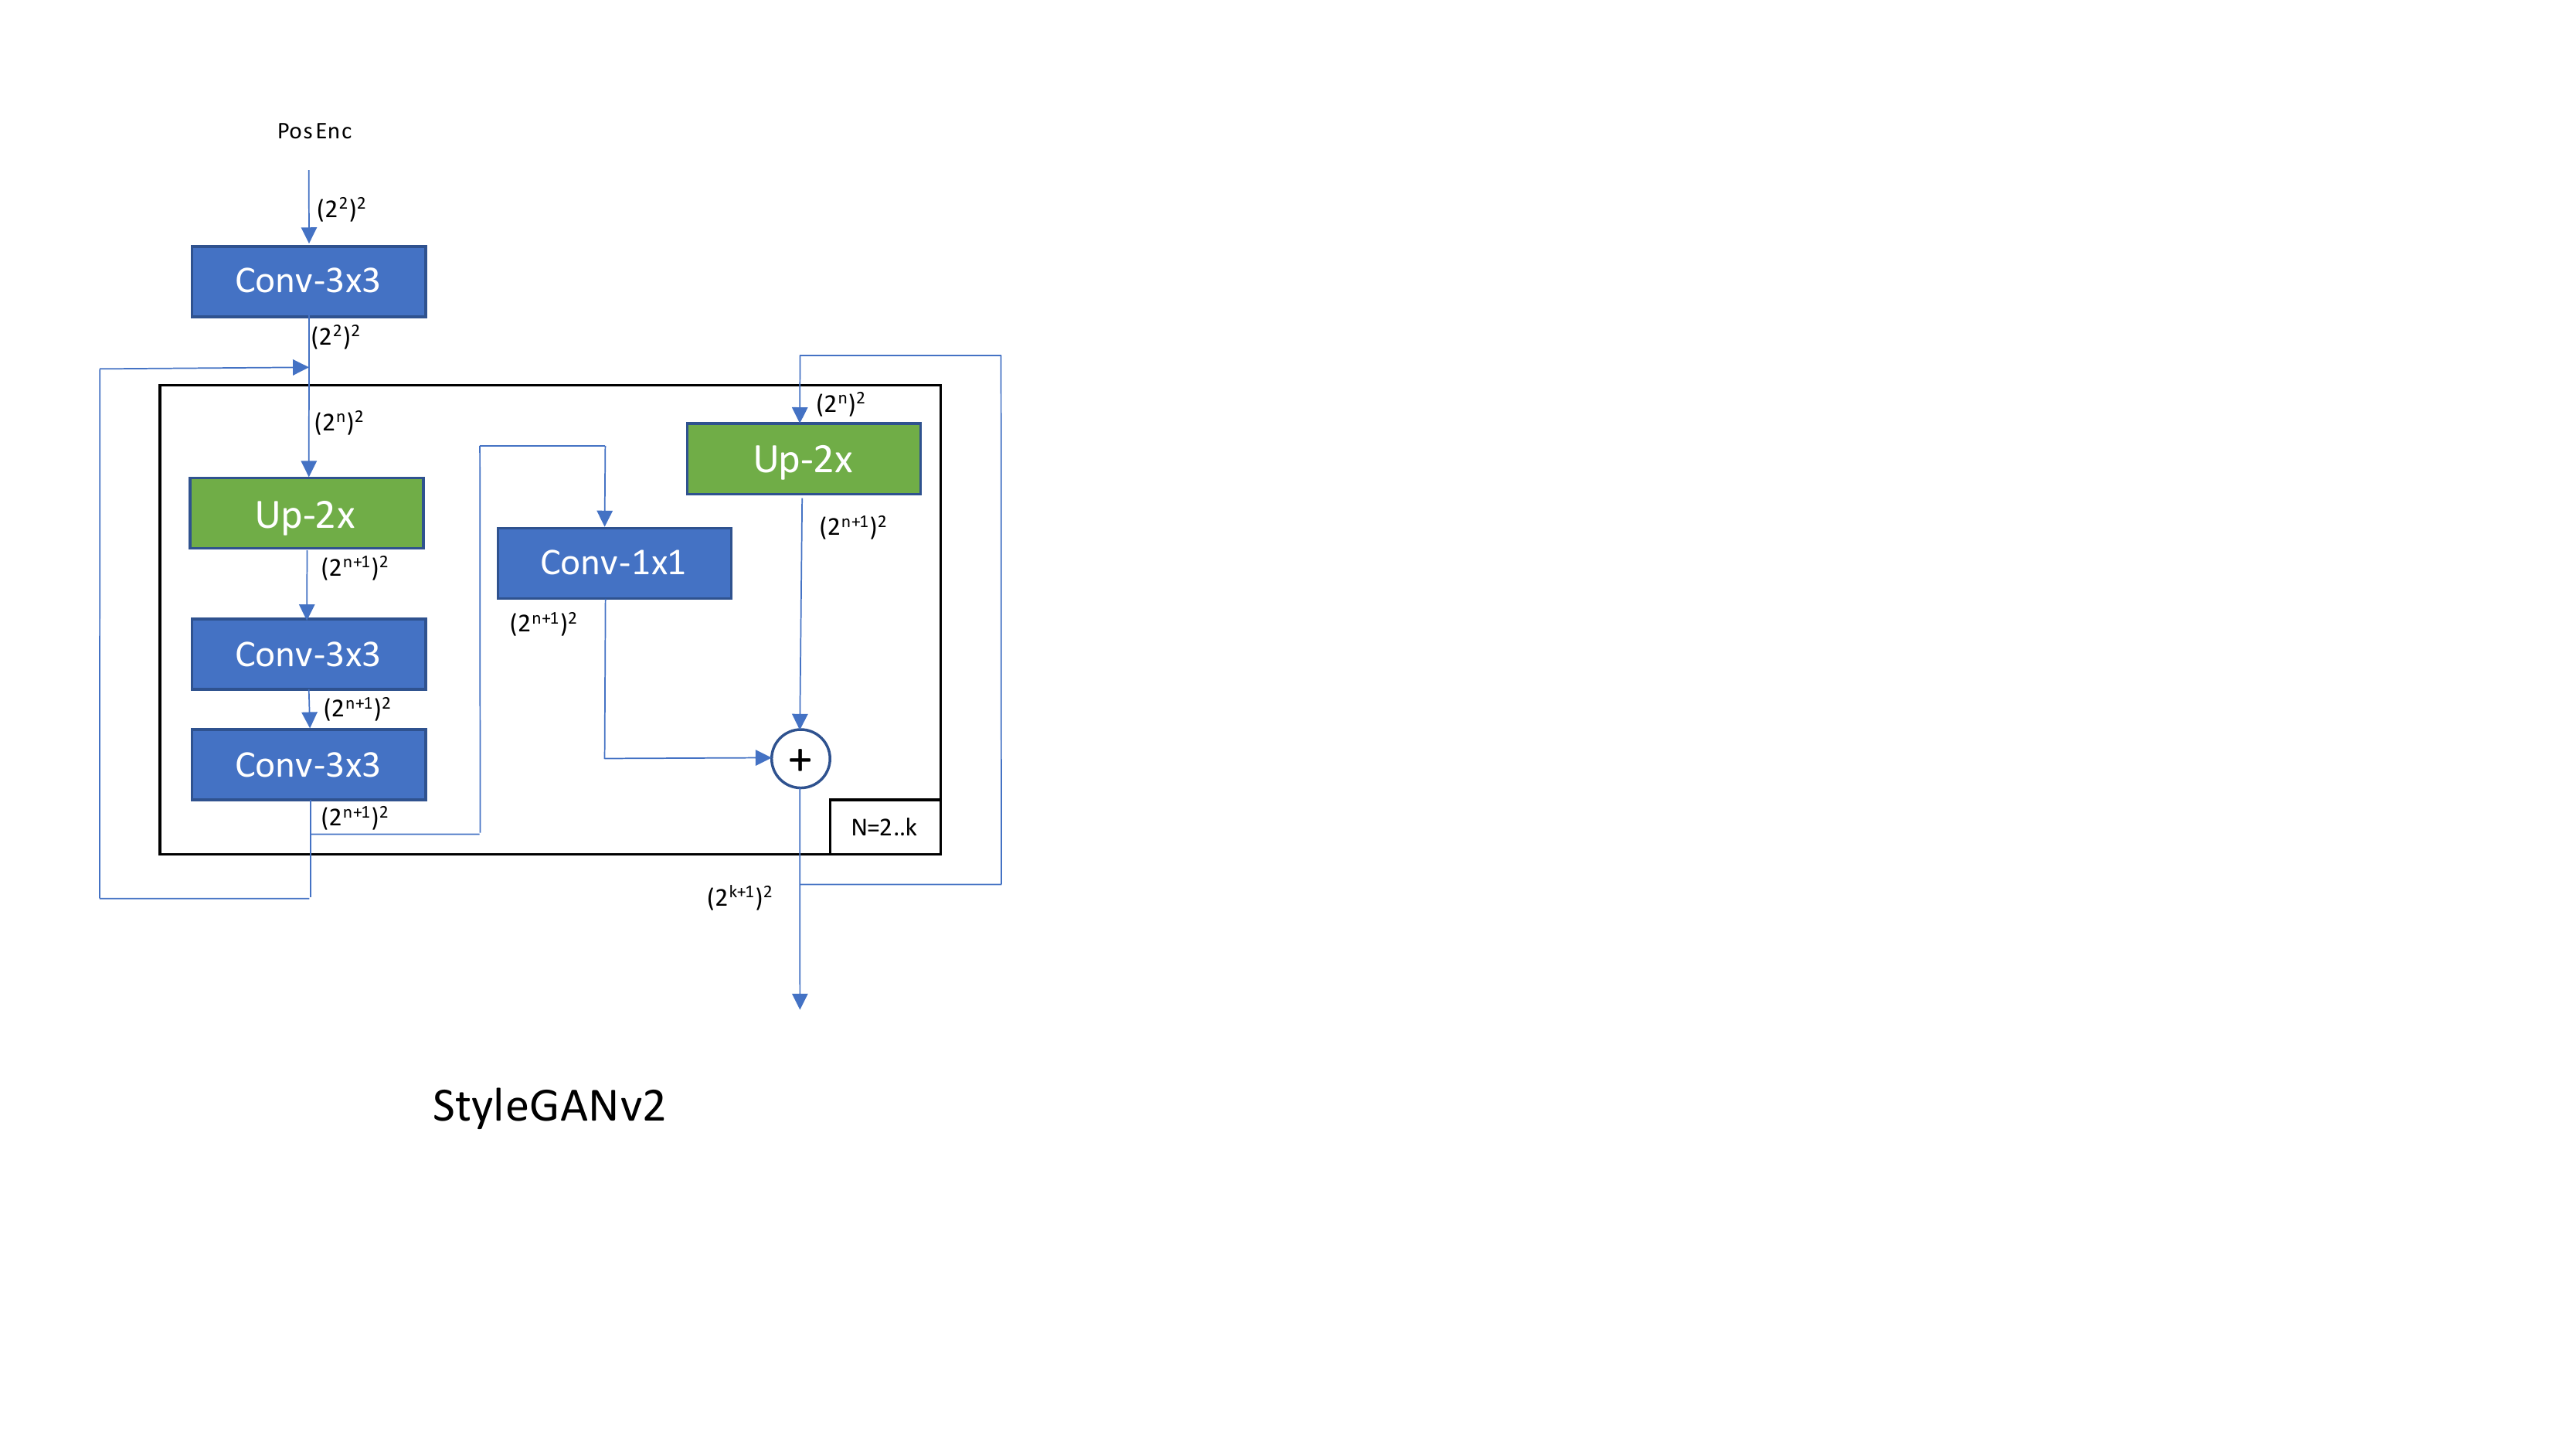} &
         \includegraphics[width=0.30\linewidth, trim=40 110 570 50, clip]{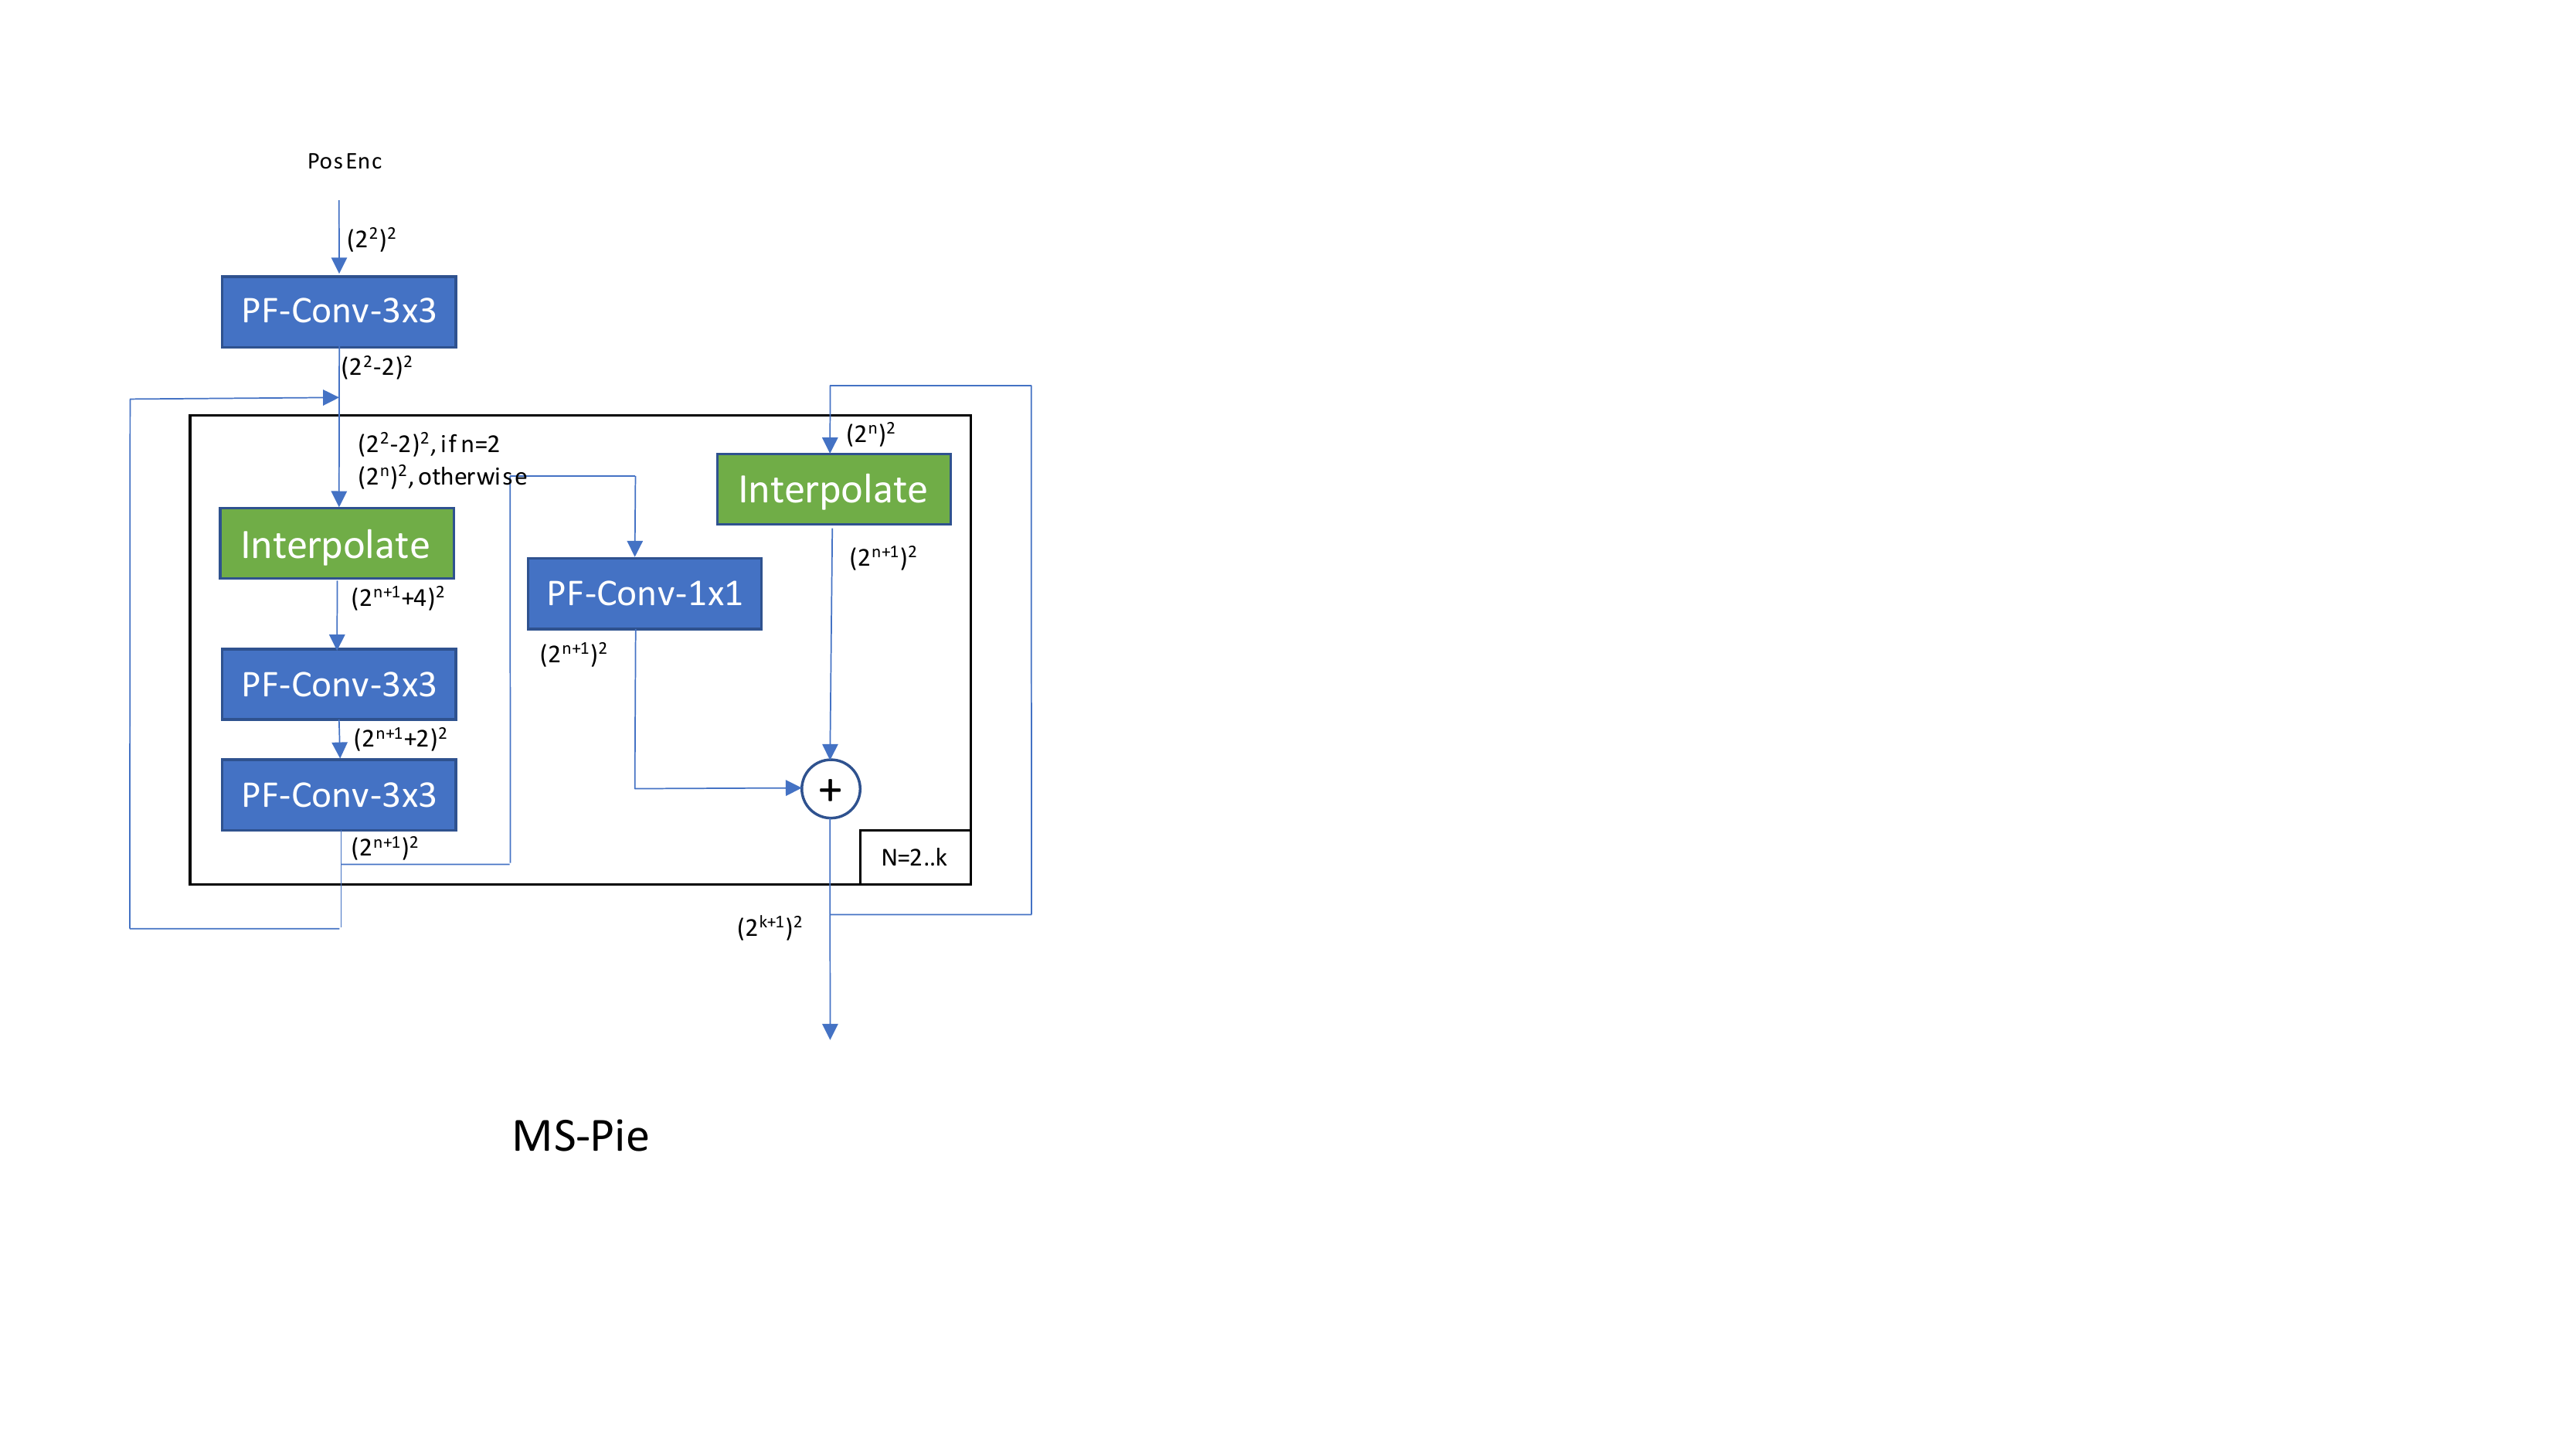} &
         \includegraphics[width=0.30\linewidth, trim=30 120 580 40, clip]{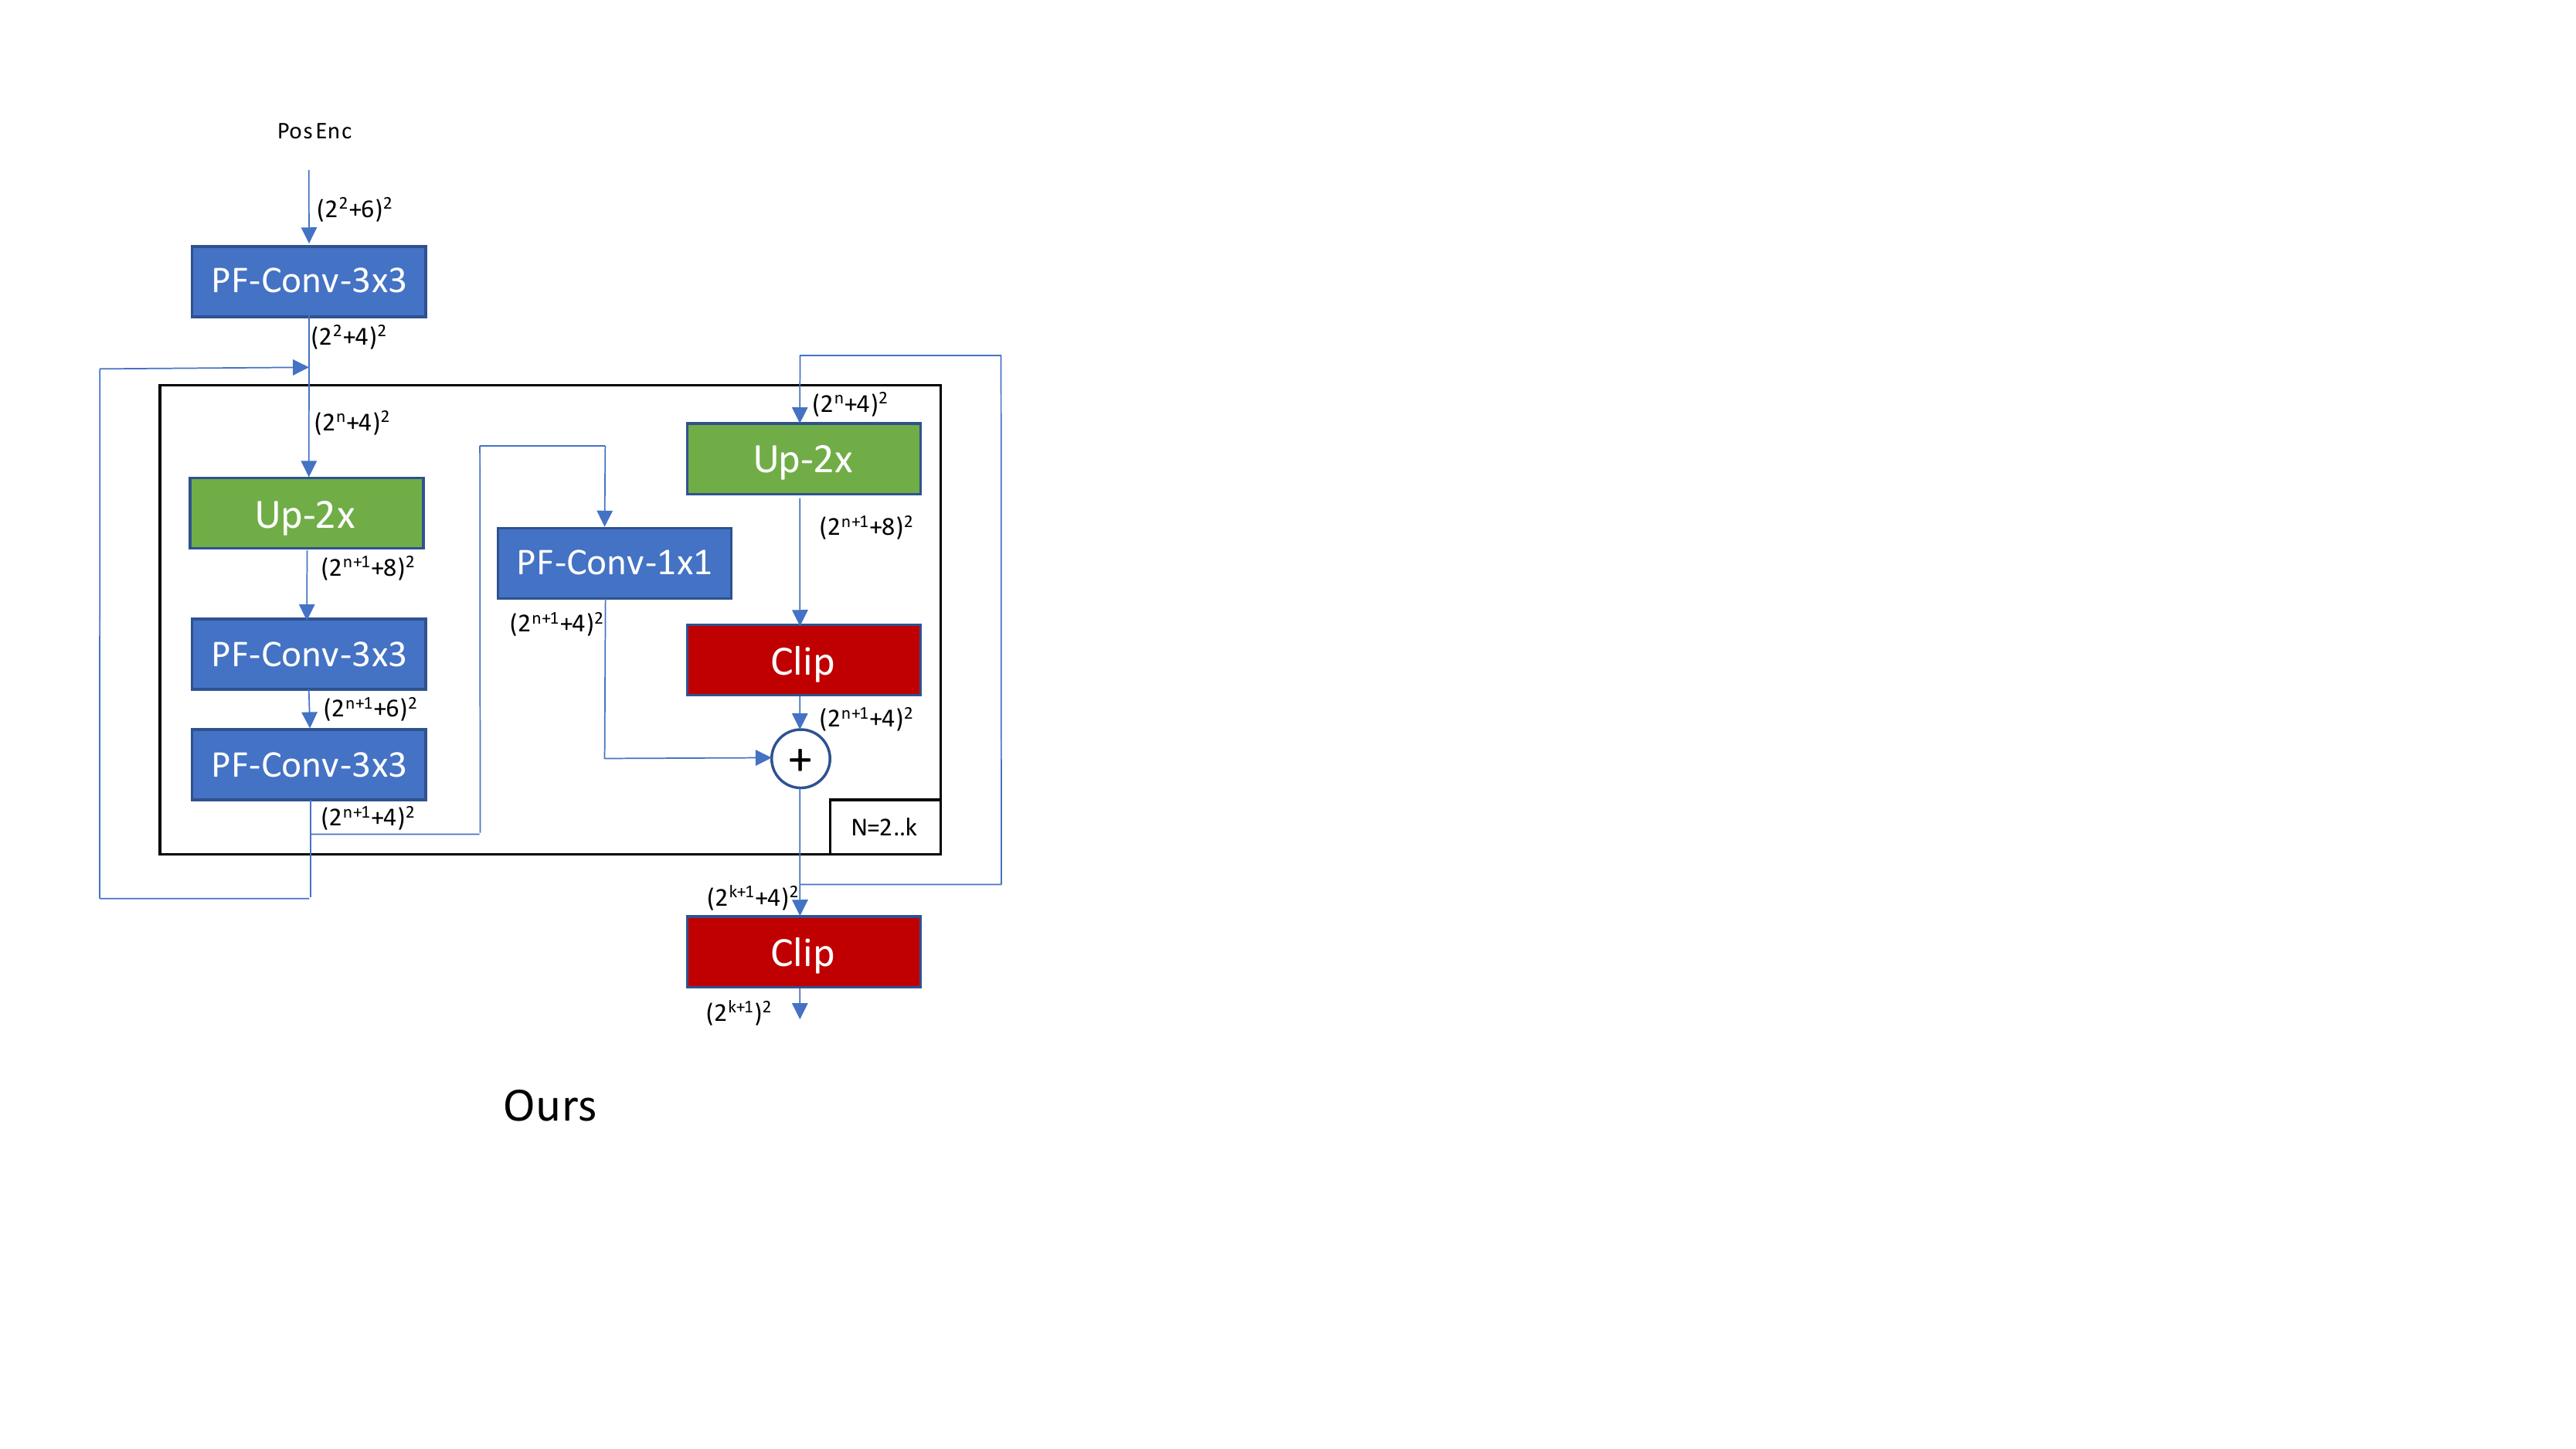} 
    \end{tabular}
    \caption{}
    \label{fig:featmap}
 
\end{figure*}

\subsection{Training only partially without full images}

    Global consistency fails, look at experiment dual_mix_half_resolution
